# Supplementary material for: Inverse Resistive Force Theory (I-RFT): Learning granular properties through robot-terrain physical interactions
Source: arXiv:2603.07796 source file (2026-03-08)
Supplement: Supplementary file 1 [file additionalandextensionstudy.tex]

\section{Additional studies and discussion} 
\subsection{Structural prior incorporation}
As established in~\cite{lichenrft}, the stress per unit depth map $\alpha_{z,x}(\beta, \gamma)$ is generic across dry homogeneous granular media, differing only by a scaling factor $\zeta$. To leverage this prior information, we model terrain-specific stresses as a scaled generic profile plus a GP residual with the initial assumption of dry homogeneous media. Specificalzly, we decompose each stress per unit depth map as:
\begin{align}
\alpha_z(\theta) &= \zeta_z \cdot \alpha_{\text{base},z}(\theta) + r_z(\theta), \nonumber \\
&\quad r_z(\cdot) \sim \mathcal{GP}(0, k_z(\cdot, \cdot)), \\
\alpha_x(\theta) &= \zeta_x \cdot \alpha_{\text{base},x}(\theta) + r_x(\theta), \nonumber \\
&\quad r_x(\cdot) \sim \mathcal{GP}(0, k_x(\cdot, \cdot)),
\end{align}
where $\alpha_{\text{base},z}(\theta)$ and $\alpha_{\text{base},x}(\theta)$ are the known generic profiles reported in~\cite{lichenrft}, $\zeta_z$ and $\zeta_x$ are terrain-specific scaling factors, and $r_z(\theta)$ and $r_x(\theta)$ are residual GP functions using the same kernel structure as defined in Sec. \ref{sec-gaussian}.

Substituting this decomposition into the composite observation model (Eq.~\eqref{eq:rft_sensor_integration}), each torque observation becomes a combination of the scaled base profile contribution and the residual GP evaluations. We define residual observations as $\mathbf{y}(\zeta) \triangleq \boldsymbol{\tau}_t - \boldsymbol{\tau}_{\text{base}}(\zeta)$, where $\boldsymbol{\tau}_{\text{base}}(\zeta)$ is the torque predicted by the scaled generic profile alone. The residual model then follows the same composite observation structure as before: $\mathbf{y} \sim \mathcal{N}(\mathbf{0}, C)$ where $C = W_z K_z W_z^\top + W_x K_x W_x^\top + \sigma_n^2 I$ (same as Eq.~\eqref{eq:joint_distribution_composite}).

In practice, we fit this semi-parametric model hierarchically. In the \emph{first stage}, we set $r_z = r_x = 0$ and estimate the scaling factors by minimizing the discrepancy between the measured torques and the torques predicted by the scaled base profile,
\begin{equation}
(\hat{\zeta}_z, \hat{\zeta}_x)
= \arg\min_{\zeta_z, \zeta_x}
\big\|\boldsymbol{\tau}_t - \boldsymbol{\tau}_{\text{base}}(\zeta)\big\|_2^2,
\end{equation}
which is equivalent to maximum likelihood under a Gaussian noise model with no residual GP. In the \emph{second stage}, we fix $\zeta = \hat{\zeta}$ and treat $\mathbf{y}(\hat{\zeta})$ as observations of the residual GP, using the composite covariance $C$ defined above. The residual GP hyperparameters $\psi = \{\ell_z, \ell_x, \sigma_{f,z}, \sigma_{f,x}, \sigma_{n, z}, \sigma_{n, x}\}$ are then optimized following Eqn. \ref{eq:marginal_log_likelihood}. 

This hierarchical formulation is designed to be numerically stable and interpretable: the scaling factors $\hat{\zeta}_z$ and $\hat{\zeta}_x$ capture global material strength with the assumption of dry homogeneous media, while the residual GP is used only to discover new effects in an unknown granular terrain from the RFT prior, such as anisotropy, cohesion, saturation effects, or other non-RFT behaviors.

% \subsection{Active Learning to Improve Performance}
% Based on the derivations above, obtaining a more accurate stress map requires that, during data collection, we acquire angle parameters $\theta$ that are distributed as broadly as possible. This guides how we choose the leg shape and motion mode so as to maximize data efficiency.

\subsection{Incorporating strong priors and hypothesis verification}
\subsection{4. Incorporating Structured Priors into a Semi-Parametric Residual GP}

To enhance model robustness and interpretability, we incorporate structured prior information derived from prior terrain knowledge or a reference model. We define:

\[
f(\theta) = a \cdot f_{\text{base}}(\theta) + r(\theta), \quad r(\cdot) \sim \mathcal{GP}(0, k(\cdot, \cdot)),
\]

where the residual function $r(\theta)$ captures deviations from the base function. The composite observations then become:

\[
y_i = \sum_{m=1}^{M} w_{i,m}[a \cdot f_{\text{base}}(\theta_{i,m}) + r(\theta_{i,m})] + \varepsilon_i.
\]

Letting $\mathbf{f}_{\text{base}}$ represent the vector of base function evaluations and $\mathbf{r}$ the residual latent function, we express the marginal log-likelihood as:

\begin{align}
\log p(\mathbf{y}_t \mid a)
&= -\frac{1}{2} 
    (\mathbf{y}_t - a W\mathbf{f}_{\text{base}})^\top \nonumber \\
&\quad \cdot (W K W^\top + \sigma_n^2 I)^{-1}
    (\mathbf{y}_t - a W\mathbf{f}_{\text{base}}) \nonumber \\
&\quad - \frac{1}{2} 
    \log \!\left| W K W^\top + \sigma_n^2 I \right| 
    - \frac{t}{2} \log(2\pi).
\end{align}

Optimizing this likelihood jointly over the scaling factor $a$ and GP hyperparameters yields a flexible and adaptive model. This approach explicitly quantifies structured deviations from prior knowledge, providing valuable insights into the validity and applicability of the prior.

\subsection{Active trajectory design and shape selection}
{\SL more ablation study comes here}

\section{Real Robot experiments}
{\SL needs an image for the Real Robot setup and comparisons}
\subsection{Experiments of customized motion primitives}
\subsubsection{Traveler robotic leg}
\subsubsection{Experiment setup}
\subsubsection{Estimation results}
\subsubsection{Analysis}
\subsection{Experiments of C-shape leg and rotating motion primitives}

\subsection{Proprioceptive Sensory Modeling}

During locomotion, we observe proprioceptive measurements as motor torques \(\boldsymbol{\tau} = [\tau_1, \tau_2, \dots, \tau_N]^\top\), a vector of observed torque estimations where each element corresponds to a motor, estimated from motor current using the torque constant~\cite{kenneally2016design}. External contact forces \(\mathbf{F}_{\text{external}} = [f_x, f_z]^\top\) acting on the robot are transformed through the robot's kinematic Jacobian \(\mathbf{J}\) to produce these joint-level torques:
\begin{equation}
\boldsymbol{\tau} = \mathbf{J}^{\top} \mathbf{F}_{\text{external}}
\label{eq:jacobian_transform}
\end{equation}
where \(\mathbf{F}_{\text{external}}\) represents contact forces in the robot frame. The Jacobian derivation for the four robot configurations used in this paper is provided in Appendix~\ref{app:jacobian}.

To integrate this sensory model with RFT, the joint torques \(\boldsymbol{\tau}\) arise from the integral of local stress contributions across all contact segments, each transformed through its segment-specific Jacobian:
\begin{equation}
\boldsymbol{\tau} = \sum_{m=1}^{M} |z_m| A_m \, \mathbf{J}_m^{\top} \begin{bmatrix} \alpha_z(\beta_m, \gamma_m) \\ \alpha_x(\beta_m, \gamma_m) \end{bmatrix}
\label{eq:rft_sensor_integration}
\end{equation}
where \(\mathbf{J}_m \in \mathbb{R}^{2 \times N}\) is the Jacobian for the \(m\)-th segment (mapping 2D contact forces to \(N\) joint torques), and \(\boldsymbol{\tau} \in \mathbb{R}^{N}\) is the vector of joint torques. During interaction, \(|z_m|\), \(A_m\), and \(\mathbf{J}_m\) are known from the robot's state and contact geometry, while they vary with segment and robot configuration. 

The Jacobian transformation couples the vertical and horizontal stress components: each torque observation \(\tau_i\) is a linear combination of both \(\alpha_z\) and \(\alpha_x\) evaluated at multiple segments. While we model \(\alpha_z\) and \(\alpha_x\) as independent Gaussian processes, the joint torque observations require solving them jointly, as the Jacobian matrix \(\mathbf{J}_m\) simultaneously transforms both force components into the observed torques. This formulation couples the RFT forward model with the proprioceptive sensor model, forming a linear inverse problem to infer the latent stress per unit depth maps \(\alpha_z(\beta, \gamma)\) and \(\alpha_x(\beta, \gamma)\) from joint-level torque observations \(\boldsymbol{\tau}\).

\newpage
\appendix

\section{Jacobian Derivation}
\label{app:jacobian}

This appendix provides the Jacobian derivation for the four robot configurations used in this paper. The Jacobian matrix relates joint-level torques to end-effector forces, enabling the transformation from proprioceptive measurements to contact forces.

\subsection{Traveler Leg Configuration}

For the Traveler leg configuration, the Jacobian derivation follows the kinematic relationships shown in Fig.~\ref{fig:traveler}. The end-effector position \((x, y)\) is expressed in terms of the composite length \(l\) and angle \(\theta\):
\[
x = l \sin(\theta), \quad y = l \cos(\theta),
\]
where \(l = l_3 + l_1 \cos(\gamma) + \sqrt{l_2^2 - l_1^2 \sin^2(\gamma)}\), and the angles are defined as:
\[
\theta = \frac{1}{2}(\phi_1 + \phi_2), \quad \gamma = \frac{1}{2}(-\phi_1 + \phi_2),
\]
with \(\phi_1\) and \(\phi_2\) being the joint angles.

The differential kinematics relating end-effector position to joint angles is:
\[
\begin{bmatrix} dx \\ dy \end{bmatrix} = \mathbf{J} \begin{bmatrix} d\phi_1 \\ d\phi_2 \end{bmatrix},
\]
where the Jacobian matrix \(\mathbf{J}\) is:
\[
\mathbf{J} = \frac{1}{2} \begin{bmatrix}
-\Phi \sin(\theta) + l \cos(\theta) & \Phi \sin(\theta) + l \cos(\theta) \\
-\Phi \cos(\theta) - l \sin(\theta) & \Phi \cos(\theta) - l \sin(\theta)
\end{bmatrix},
\]
with \(\Phi = -l_1 \sin(\gamma) \left(1 + \frac{l_1 \cos(\gamma)}{\sqrt{l_2^2 - l_1^2 \sin^2(\gamma)}}\right)\).

Using the principle of virtual work, the relationship between end-effector forces and joint torques is:
\[
\begin{bmatrix} F_x \\ F_y \end{bmatrix} = \begin{bmatrix} \tau_1 \\ \tau_2 \end{bmatrix} \mathbf{J}^{-1},
\]
where \(F_x\) and \(F_y\) are the leg forces exerted on the substrate, and \(\tau_1\) and \(\tau_2\) are the joint torques. This result does not include gravity compensation.

\subsection{Other Configurations}

The Jacobian derivations for the remaining three robot configurations (C-leg rotation, plate toe with Traveler leg, and C-toe with Traveler leg) follow similar principles, with the specific kinematic relationships depending on each configuration's geometry and degrees of freedom.

\subsection{Proprioceptive Sensory Modeling}

During locomotion, we observe proprioceptive measurements as motor torques \(\boldsymbol{\tau} = [\tau_1, \tau_2, \dots, \tau_N]^\top\), a vector of observed torque estimations where each element corresponds to a motor, estimated from motor current using the torque constant~\cite{kenneally2016design}. External contact forces \(\mathbf{F}_{\text{external}} = [f_x, f_z]^\top\) acting on the robot are transformed through the robot's kinematic Jacobian \(\mathbf{J}\) to produce these joint-level torques:
\begin{equation}
\boldsymbol{\tau} = \mathbf{J}^{\top} \mathbf{F}_{\text{external}}
\label{eq:jacobian_transform}
\end{equation}
where \(\mathbf{F}_{\text{external}}\) represents contact forces in the robot frame. The Jacobian derivation for the four robot configurations used in this paper is provided in Appendix~\ref{app:jacobian}.

To integrate this sensory model with RFT, the joint torques \(\boldsymbol{\tau}\) arise from the integral of local stress contributions across all contact segments, each transformed through its segment-specific Jacobian:
\begin{equation}
\boldsymbol{\tau} = \sum_{m=1}^{M} |z_m| A_m \, \mathbf{J}_m^{\top} \begin{bmatrix} \alpha_z(\beta_m, \gamma_m) \\ \alpha_x(\beta_m, \gamma_m) \end{bmatrix}
\label{eq:rft_sensor_integration}
\end{equation}
where \(\mathbf{J}_m \in \mathbb{R}^{2 \times N}\) is the Jacobian for the \(m\)-th segment (mapping 2D contact forces to \(N\) joint torques), and \(\boldsymbol{\tau} \in \mathbb{R}^{N}\) is the vector of joint torques. During interaction, \(|z_m|\), \(A_m\), and \(\mathbf{J}_m\) are known from the robot's state and contact geometry, while they vary with segment and robot configuration. 

The Jacobian transformation couples the vertical and horizontal stress components: each torque observation \(\tau_i\) is a linear combination of both \(\alpha_z\) and \(\alpha_x\) evaluated at multiple segments. While we model \(\alpha_z\) and \(\alpha_x\) as independent Gaussian processes, the joint torque observations require solving them jointly, as the Jacobian matrix \(\mathbf{J}_m\) simultaneously transforms both force components into the observed torques. This formulation couples the RFT forward model with the proprioceptive sensor model, forming a linear inverse problem to infer the latent stress per unit depth maps \(\alpha_z(\beta, \gamma)\) and \(\alpha_x(\beta, \gamma)\) from joint-level torque observations \(\boldsymbol{\tau}\).

1. analysis of different noise levels.
